# Supplementary material for: Recovering Latent Confounders from High-dimensional Proxy Variables
Source: arXiv:2403.14228 source file (2024-03-21)
Supplement: Supplementary file 1 [file original_submission_supp.tex]

\section{Dimensionality Reduction}
\label{app:dr}
For the synthetic example, we use the R packages {\tt prcomp} implementation of PCA, {\tt fastICA} package for ICA, and {\tt mdatools} package for PLS.
For the common driver example, we use Python packages {\tt Scikit-learn} implementations of PCA, {\tt PLSSVD} for PLS regression, and {\tt FastICA} for ICA.

\paragraph{More on PCA and PLS}
As stated earlier in this section, PCA and PLS both result in truncated orthogonal estimates for $\mathbf{V}$ as $\widehat{\mathbf{V}}$. In both cases these estimates satisfy $\widehat{\mathbf{V}}^T \widehat{\mathbf{V}} = \mathbf{I}$, but order the columns of $\widehat{\mathbf{V}}$ differently than the ordering in Eq.~\eqref{eq:gen_loss_fxn}. Therefore, we do not expect PCA or PLS to consistently recover the correct latent confounders up to a permutation. Specifically, in PCA, we order these columns in terms of increasing explained variance
\begin{equation}
    \mathbf{v}_1^T \mathbf{C}_\mathbf{U} \mathbf{v}_1 \geq \mathbf{v}_2^T \mathbf{C}_\mathbf{U} \mathbf{v}_2 \geq \cdots \geq \mathbf{v}_k^T \mathbf{C}_\mathbf{U} \mathbf{v}_k \geq 0,
\end{equation}
and in PLS, the columns are ordered differently, as
\begin{equation}
     \mathbf{v}_1^T \mathbf{C}_{\mathbf{U},\widetilde{\mathbf{X}}} \widetilde{\mathbf{v}}_1 \geq \mathbf{v}_2^T \mathbf{C}_{\mathbf{U},\widetilde{\mathbf{X}}} \widetilde{\mathbf{v}}_2 \geq \cdots \geq \mathbf{v}_k^T \mathbf{C}_{\mathbf{U},\widetilde{\mathbf{X}}} \widetilde{\mathbf{v}}_k \geq 0.
\end{equation}

\section{PCF with PC Algorithm}

\begin{figure}[h!]
    \centering
    \includegraphics[width=0.8\textwidth]{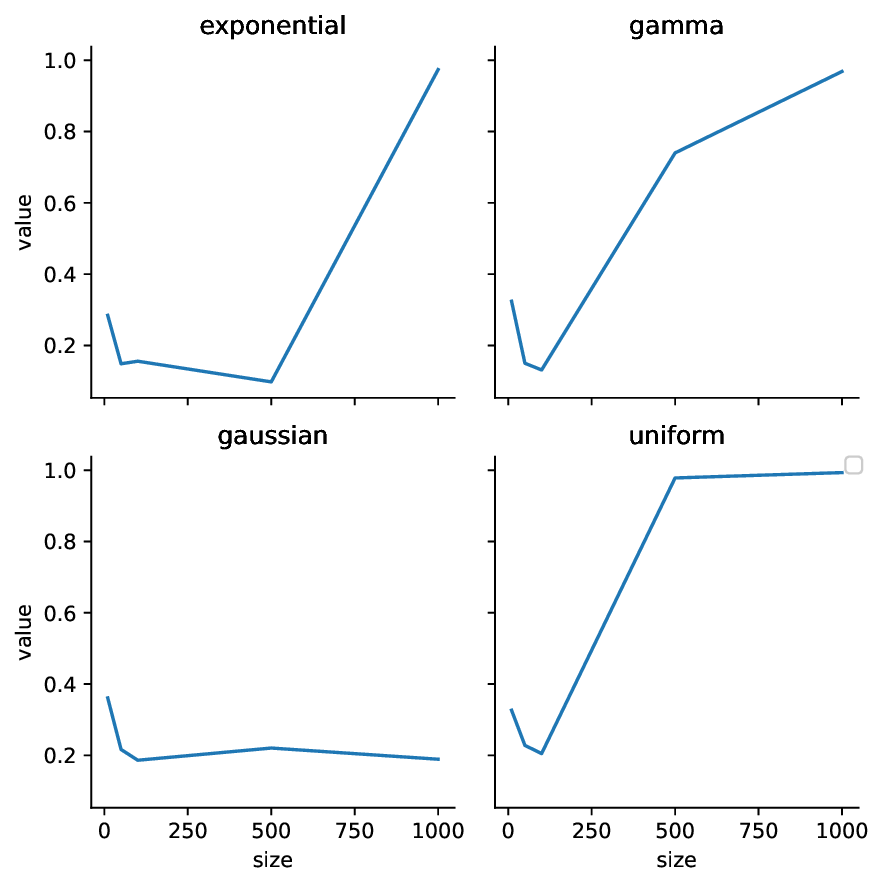}
    \caption{Performance of ICA-PCF implementation on synthetic data when instead of using our $p$-value regression-based selection criterion, we use the PC-algorithm.}
    \label{fig:ICA_PC}
\end{figure}

Figure \ref{fig:ICA_PC} shows the results of the ICA-PCF implementation on synthetic data when we use the PC-algorithm \cite{PCalgo} to select the confounding variable from those produced by ICA. All assumptions encoded in the DAG shown in Figure \ref{fig:dag_scm} are introduced as prior knowledge so that the PC algorithm is only used to evaluate possible directed edges from the components of $\hat{\mathbf{Z}}$ to $x$ and $y$. We select as confounding components of $\hat{\mathbf{Z}}$ those having edges to both $x$ and $y$. Since we assume $z_c$ is univariate, we adjust the hyperparameter significance level $\alpha$ for the individual conditional independence tests performed by the PC algorithm in order to obtain as output a single confounding variable. Since we are in a linear setting, we base the conditional independence test on partial correlation. When comparing with Figure \ref{fig:synthetic} we can see that for limited data settings, our p-value, regression-based selection criteria performs better than the PC algorithm. 

% \section{Additional results on synthetic data}
% \label{app:additional}

\section{Common driver example}
\label{app:commondriver}

As shown in Figure \ref{fig:confounder_weights_PCAPLS}, both PCA-PCF and PLS-PCF exhibit similar patterns to ICA-PCF in terms of their weights in the NAO-stations area. It is noteworthy that all three methods fail to accurately recover the NAO signal in the years 2000 to 2005. This may be attributed to the fact that precipitation patterns in both Denmark and the Mediterranean region during this period were not strongly correlated with the NAO. This should be further investigated.

\begin{figure}[h]
    \centering
    \begin{tikzpicture}[auto,  
    edge/.style ={arrows=-{Latex[length=2mm]}}]
        \node (figa) at (0,0) {\includegraphics[width=0.45\textwidth]{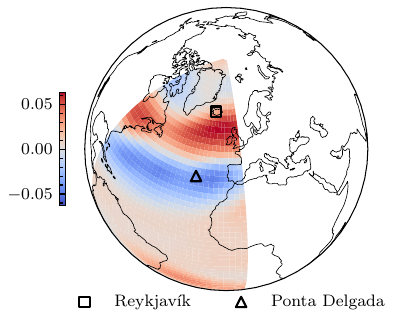}};
        \node (a) at (-2.5,2.5) {\bf PCA-PCF};
        \node (figb) at (6.5,0) {\includegraphics[width=0.45\textwidth]{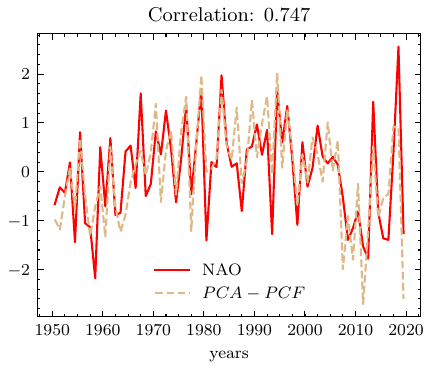}};
        \node (b) at (3,2.5) {};

        \node[circle, draw, fill=lightgray, inner sep=0.4pt, minimum size = 16pt] (dk) at (0.8, 0.6) {\tiny \textbf{DK}};

        \node[circle, draw, fill=lightgray, minimum size = 1pt, inner sep=0.1pt] (med) at (0.9, -0.2) {\tiny \textbf{MED}};

        \node[circle, draw, fill=lightgray, minimum size = 16pt, inner sep=0.1pt] (nao) at (-0.1, 0.2) {\tiny \textbf{NAO}};

            \path[edge, color = black, line width=1pt] (nao) edge (dk);

            \path[edge,
            color = black, line width=1pt] (nao) edge (med);
        
    \end{tikzpicture}

    \begin{tikzpicture}[auto,  
    edge/.style ={arrows=-{Latex[length=2mm]}}]
        \node (figa) at (0,0) {\includegraphics[width=0.45\textwidth]{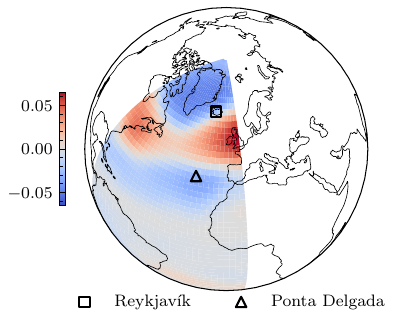}};
        \node (a) at (-2.5,2.5) {\bf PLS-PCF};
        \node (figb) at (6.5,0) {\includegraphics[width=0.45\textwidth]{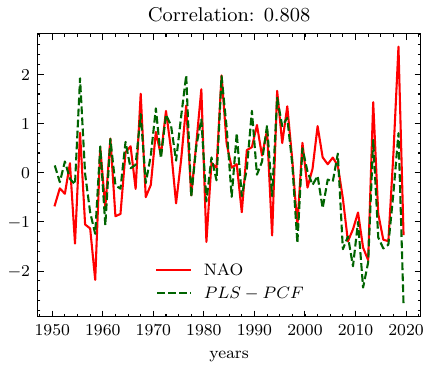}};
        \node (b) at (3,2.5) {};

        \node[circle, draw, fill=lightgray, inner sep=0.4pt, minimum size = 16pt] (dk) at (0.8, 0.6) {\tiny \textbf{DK}};

        \node[circle, draw, fill=lightgray, minimum size = 1pt, inner sep=0.1pt] (med) at (0.9, -0.2) {\tiny \textbf{MED}};

        \node[circle, draw, fill=lightgray, minimum size = 16pt, inner sep=0.1pt] (nao) at (-0.1, 0.2) {\tiny \textbf{NAO}};

            \path[edge, color = black, line width=1pt] (nao) edge (dk);

            \path[edge,
            color = black, line width=1pt] (nao) edge (med);
        
    \end{tikzpicture}
    
    \caption{Coefficient matrices $\mathbf{A}$ (right) and first confounder extracted (left) for the PCA-PCF (top) and PLS-PCF (bottom). We indicate the correlation with NAO.}
    \label{fig:confounder_weights_PCAPLS}
\end{figure}

\iffalse
\begin{figure}[h]
    \centering
    \begin{tikzpicture}[auto,  
    edge/.style ={arrows=-{Latex[length=2mm]}}]
        \node (figa) at (0,0) {\includegraphics[width=0.45\textwidth]{figures/Weights_Plot_Final_PLS.pdf}};
        \node (a) at (-2.5,2.5) {(a)};
        \node (figb) at (6.5,0) {\includegraphics[width=0.45\textwidth]{figures/Corr_Plot_Final_PLS.pdf}};
        \node (b) at (3,2.5) {(b)};

        \node[circle, draw, fill=lightgray, inner sep=0.4pt, minimum size = 16pt] (dk) at (0.8, 0.6) {\tiny \textbf{DK}};

        \node[circle, draw, fill=lightgray, minimum size = 1pt, inner sep=0.1pt] (med) at (0.9, -0.2) {\tiny \textbf{MED}};

        \node[circle, draw, fill=lightgray, minimum size = 16pt, inner sep=0.1pt] (nao) at (-0.1, 0.2) {\tiny \textbf{NAO}};

            \path[edge, color = black, line width=1pt] (nao) edge (dk);

            \path[edge,
            color = black, line width=1pt] (nao) edge (med);
        
    \end{tikzpicture}
    \caption{a) Coefficient matrix ($\mathbf{A}$) in the PLS-PCF projection.
    (b) First confounder extracted by PLS-PCF.}
    \label{fig:confounder_weights_PLS2}
\end{figure}
\fi

We provide the linear SCMs induced by each of the three DR algorithms in Figs.~\ref{fig:image1},~\ref{fig:image2}, and~\ref{fig:image3}. 
Only using ICA in PCF allows us to identify direct links from $\{Z_1,Z_2,Z_3\}$ to MED and DK. 

\begin{figure}[h]
  \centering
    \includegraphics[width=.7\linewidth]{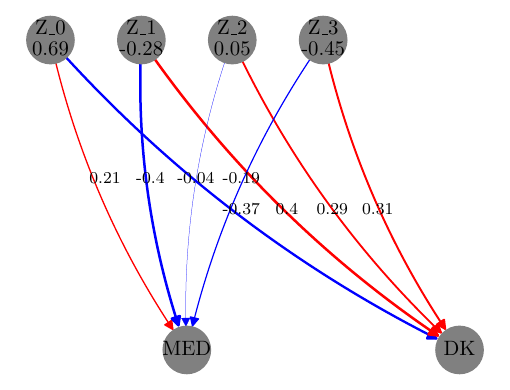}
    \caption{Causal graph generated by ICA-PCF, with the correlation to NAO indicated beneath each of the respective confounders.\label{fig:image1}}
\end{figure}

\begin{figure}[h]
    \centering
    \includegraphics[width=.7\linewidth]{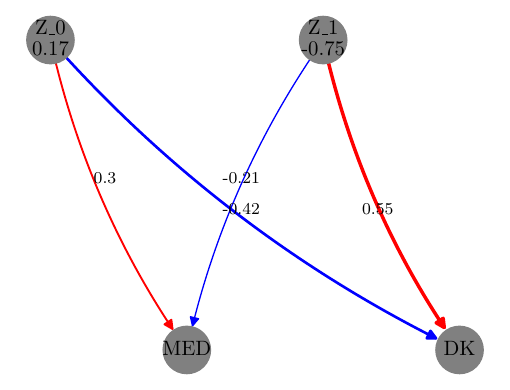}
    
    \caption{Causal graph generated by PCA-PCF, with the correlation to NAO indicated beneath each of the respective confounders.\label{fig:image2}  }
\end{figure}

\begin{figure}
    \centering
    \includegraphics[width=.7\linewidth]{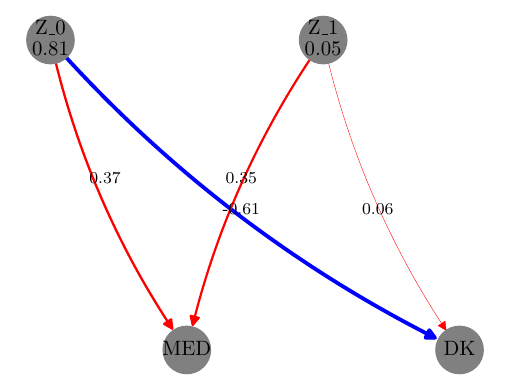}
    
  \caption{Causal graph generated by PLS-PCF, with the correlation to NAO indicated beneath each of the respective confounders.\label{fig:image3}}
\end{figure}

\newpage
